# Supplementary material for: Emergence and coexistence of periodic and unstructured motion in future-avoiding random walks
Source: arXiv:2602.03308 source file (2026-10-30)
Supplement: Supplementary file 1 [file supplement.pdf]

# Supplemental Information for: Emergence and co-existence of periodic and unstructured motion in future-avoiding random walks

A. Schmaus,[1,2] K. Stiller,[1,2] and N. Molkenthin[1,*]

[1] *Potsdam Institute for Climate Impact Research, Telegrafenberg A 31, Potsdam, Germany*

[2] *Technical University Berlin, Straße des 17. Juni 135, Berlin 10623, Germany*

(Dated: January 28, 2026)

## EXTENDED DESCRIPTION DISPATCHER ALGORITHM RIDE-POOLING SIMULATION

The No-detour Heuristic (NDH) dispatcher algorithm used in the simulations is based on the dispatcher algorithm shown in [1], extended for multiple vehicles and is included in the ridepy package [2]. The requests are drawn uniformly from the stop network. Every request consists of an origin and a destination node, drawn independently, and a time, generated in a Poisson process. The requests are processed sequentially. For each request, the dispatcher algorithm checks for routes already containing the origin node on a shortest path between two neighbouring nodes of the route. Fig. 1 visualizes four consecutive insertions with this dispatcher. If the origin is part of the route, the dispatcher algorithm checks whether the destination is also included after the origin. If origin and destination are part of the route, the route that reaches the destination fastest is selected. If the destination is not part of any route, the destination is attached at the end of all relevant routes, and again, the route with the earliest delivery time is selected. If neither origin nor destination are on any route, origin and destination are attached at the end of all available routes, and the request is assigned to the one with the earliest delivery time.

To make the simulation more comparable to real ride-pooling systems, additional constraints are implemented. A seat capacity limit $c$ can be assigned to each vehicle, meaning that a vehicle will reject a request if accepting it would exceed its seat capacity at any time. Additionally, a waiting time limit $t_{wait}^{max}$ can be imposed, meaning that if no vehicle can pick up the passenger before this limit, the request is rejected. A maximum delivery delay $t_{travel}^{max}$ constraint can be used to restrict long travel times. If no vehicle can satisfy this limit, the ride-pooling service will reject the request.

In summary, the simulation requires the following parameters: the ride-pooling stop network $n$, the number of busses $B$, the number of requests $r$, the average vehicle speed $v$, the normalized request load $x$, the seat capacity limit $c$, waiting time limit $t_{wait}^{max}$ and the maximum delivery delay $t_{travel}^{max}$. In this paper all vehicles have a seat limit of 20. For the NHD dispatcher, the maximum waiting and delivery delay is infinite, in order to serve every request. For the MFD dispatcher the maximum waiting time is five and the maximum delivery delay is two times the direct travel time (traveling from a node to a neighboring nodes takes one time unit). If not declared otherwise, the number of requests is always 100,000.

For every vehicle the simulation creates a route file, which contains all stops of the vehicle and which request

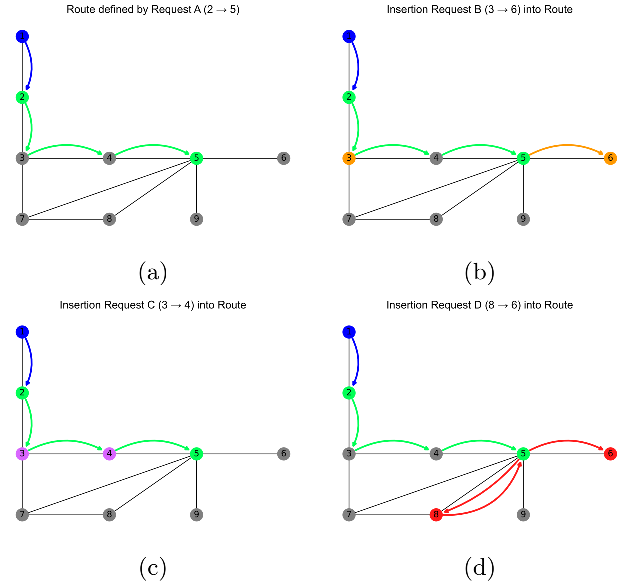


FIG. 1: Example dispatcher algorithm. Each subfigure shows vehicle position (blue) and the current route (green). The current route is defined by the shortest path from 2 to 5, the pick-up and drop-off nodes of request A. In (b) request B, from 3 to 6, is inserted. The pick-up is located on the current route, requiring no detour. The drop-off is added ad the end. In (c) the request C, from 3 to 4, is inserted into the current route. Here, the pick-up and the drop-off are part of the route, thus, both could be inserted into the current route. In (d) the request D, from 8 to 6, must be added at the end of the route, as the pick-up is not on a shortest path from 2 to 5. Here, the dispatcher rejects the optimal route (2,3,7,8,5,6) in terms of driven distance, as the optimal route would imply additional travel time for request A.

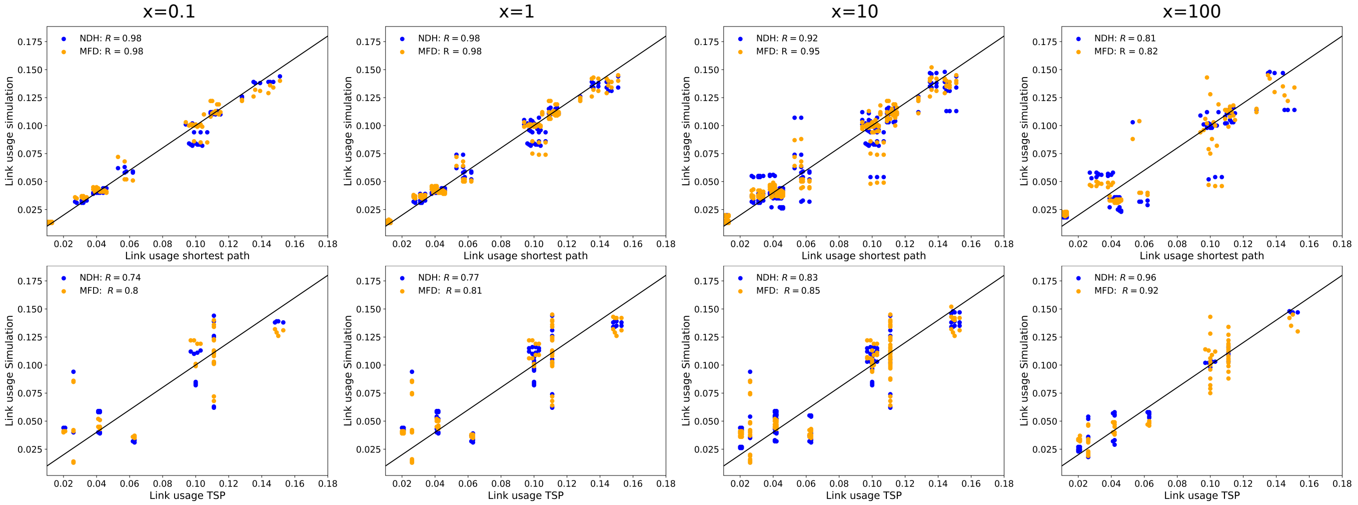


FIG. 2: Correlations of link usage to shortest path walk link usage and TSP link usage for x=0.1, x=1, x=10 and x=100. While at low x the correlation with SPW link usage is stronger, at high x, the link usage of TSP tours explains the simulated link usage better.

was fetched or delivered there. This data is used to analyze the routes of each vehicle.

## LINK USAGE FOR DIFFERENT LOADS

In the main paper we showed the correlation of pooled route link usage to both, randomized combinations of TSP tour paths and shortest path walks. For $x = 100$ we found that The former correlates better with simulation results. In Fig. 2, we extend this analysis to other values of the system load, namely $x = \{0.1, 1, 10, 100\}$.

As expected, we find that betweenness centrality correlates almost perfectly with the simulated link usage for small $x$. As $x$ increases, this correlation decreases in favour of a better correlation with link usages from randomized combinations of TSP tour paths.

## PROBABILITY DISTRIBUTION OF ROUTE PERIODICITY FRACTION

The route periodicity fraction $F$ shown in Fig.4 of the main manuscript across loads $x = \{0.1, ..., 20\}$ shows how periodic trajectories start appearing for larger loads. In Fig.3 we show the probability distributions of $F$ across the fleet, averaged over 5 realizations for $x = 20$ for both dispatchers. The probability distributions of star and cayley tree are strongly peaked at low values, followed by a steep decline for both dispatchers. The same is true for the distribution on the grid for the MDH dispatcher. This indicates the absence of periodic routes.

All other distributions reach or exceed $F \approx 1$, indicating long tails. Note that many of the distributions could be called bi- or multi-modal, with one peak at very low $F$ and another at $F \geq 0.9$. We interpret this as an indication for the co-existence of a few strongly periodic routes with a larger number of unstructured ones.

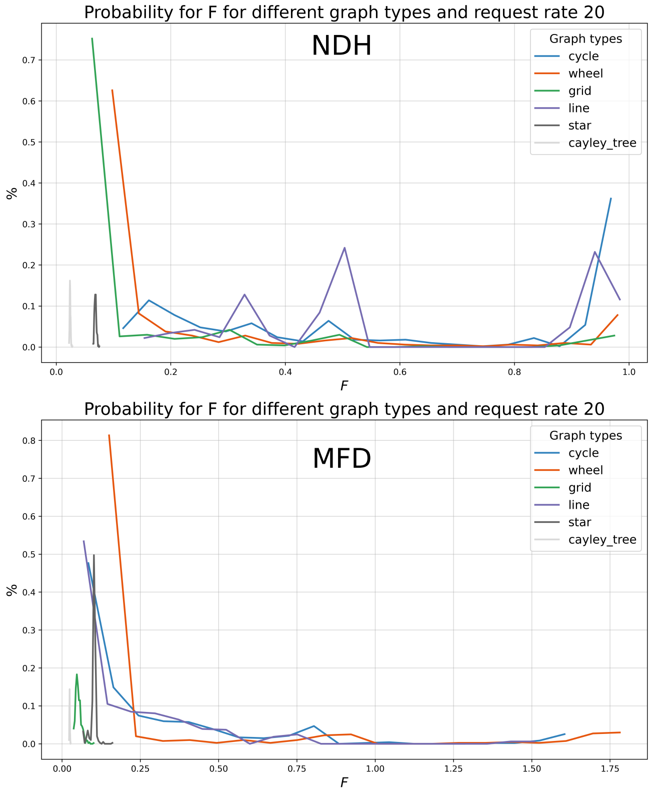


FIG. 3: Route periodicity fractions at high loads on different networks. a) For NDH dispatcher, b) For MFD dispatcher.

## THEORETICAL APPROXIMATION ON THE CYCLE GRAPH

Periodic routes emerge on four of the six networks. Here we analyze this transition in more detail by building an analytic approximation for the process based on the NDH dispatcher on the ring.

A direction change occurs if and only if a request can be served earlier by the nearest off-direction vehicle than by the nearest in-direction vehicle

$$t_s^{off} = t_w^{off} + t_d^{direct} + 2t_{over} < t_s^{in} = t_w^{in} + t_d^{direct}. \quad (1)$$

Where the waiting times for both routes are drawn from the same probability distribution $P^{wait}(t)$ and $t_{over}$ is the time it takes to drive to the end of the previously planned route from the requested pick-up point. Note that the time it takes to drive the entire planned route is $l_{route}/v$, which can be split in the part before pick up $t_w^{off}$ and the part after pick up $t_{over}$, resulting in $t_w^{off}+t_{over} = l_{route}/v$. If this is inserted into Eq.1 and simplified, we get the condition

$$t_w > l_{route}/v \quad (2)$$

for a direction change of a route. Note that this neglects direction changes of the current routes. However, we are primarily looking for the transition from fully periodic to one direction change, which limits the likelihood of pre-existing direction changes being part of a route. Drawing $t_w$ and $\langle l_{route}\rangle$ independently from their respective probability distributions, we try to find

$$P_c = P(t_w > l_{route}/v). \quad (3)$$

The waiting times are drawn from the distance distribution of $B/2$ neighbouring randomly distributed points on a ring of length $2M = N_{nodes}$

$$P(s) = \frac{\frac{B}{2}-1}{2M}(1-\frac{s}{2M})^{\frac{B}{2}-2}, \quad (4)$$

and then divided by the driving speed $v$.

At load $x$, and large fleet sizes, the occupancy at any given time approaches $O \approx x$, as shown in [3]. Thus, we approximate the current planned route as $x$ overlapping requests, one starting every $\Delta\tau$. The planned route length is therefore approximated as the maximum of drawing $x$ times from the distances between two uniformly random points and each time subtracting $i\Delta\tau v$ for values of $i \in \{1, ..., \lceil x \rceil\}$. This leads to the probability distribution

$$P(W < w) = \prod_{i=1}^{\lceil x \rceil} \frac{w + iv\Delta\tau}{M} \quad (5)$$

for drawing a value $W$ smaller than a given $w$. Combining this, we get the probability distribution

$$P_c = P(W < s) = \int_0^{2M} \prod_{i=1}^{\lceil x \rceil} \frac{s+iv\Delta\tau}{M} \frac{\frac{B}{2}-1}{2M}(1-\frac{s}{2M})^{\frac{B}{2}-2} ds, \quad (6)$$

which can be evaluated numerically (solid black line in Eq. 5 a) in the main paper) and represents the probability for one route to schedule a reversal, when including a new request.

In other words, the routes that tend to schedule a reversal are typically the shorter routes. This intuitively already explains the mechanism by which periodic routes are formed. The longer a route, the more likely new additions will preserve its direction. If a route already has a direction change scheduled, it is less likely to get assigned new requests as long as the detour is still part of the route, leading to it remaining shorter and thus more prone to direction changes.

When we repeat this process for a number of $r$ requests for each of the $B$ routes in the fleet, we can compute the probability that at least one route never changes direction as

$$P_p = 1 - (1-(1-P_c)^r)^B. \quad (7)$$

To find the steepest point we approximate it with the point at which

$$P_P = 1 - \frac{1}{e} \approx 0.6. \quad (8)$$

Inserting this simplifies Eq.7 to

$$(1-P_c)^r = 1 - e^{-1/B} \approx \frac{1}{B}, \quad (9)$$

Where the last step is a Taylor expansion to first order in $\frac{1}{B}$. This implies that the slope at this point is approximately

$$\frac{dP_p}{dx}|_{x=x_c} = -Br(1-(1-P_c)^r)^{B-1}(1-P_c)^{r-1}\frac{\partial P_c}{\partial x}|_{x=x_c}$$
$$= rB^{\frac{1}{r}}\frac{\partial P_c}{\partial x}|_{x=x_c}, \quad (10)$$

Which exhibits unbounded, yet incredibly slow growth with $B$.

* nora.molkenthin@pik-potsdam.de

[1] Debsankha Manik and Nora Molkenthin. Topology dependence of on-demand ride-sharing. *Applied Network Science*, 5(1):1–16, 2020.

[2] Felix Jung and Debsankha Manik. Ridepy: A fast and modular framework for simulating ridepooling systems. *Journal of Open Source Software*, 9(97):6241, 2024.

[3] Nora Molkenthin, Malte Schröder, and Marc Timme. Scaling laws of collective ride-sharing dynamics. *Physical Review Letters*, 125(24):248302, 2020.
